# Supplementary material for: TOP-ERL: Transformer-based Off-Policy Episodic Reinforcement Learning
Source: arXiv:2410.09536 source file (2025-03-15)
Supplement: Supplementary file 1 [file R-Rebuttal.tex]

\setcounter{section}{17}
% Add this to your LaTeX preamble
\renewcommand{\thefigure}{R\arabic{figure}}
\renewcommand{\theequation}{R.\arabic{equation}}

\section{Rebuttal: Additional Discussion and Ablation Study}
%=================================================================
% 
%                 Initial Condition Enforcement
% 
%=================================================================
\subsection{Discussion of Initial Condition Enforcement}
The initial condition enforcement of trajectories generated by ProDMP \citep{li2023prodmp} is mathematically guaranteed by the definition of initial conditions in dynamic systems, as demonstrated in Figure 2(a) and the upper part of 2(b) in the \textbf{original ProDMP paper}. In Figure~\ref{fig:enforce_init_cond_box_push}, we illustrate how TOP-ERL leverages this mechanism. The figure is based on the motion trajectory of the first degree of freedom of the robot in the box-pushing task. In the critic update, we use five segments as an example.

ProDMP, as a trajectory generator, models the trajectory as a dynamic system. In TOP-ERL, the RL policy predicts ProDMP parameters, which are used to generate a force signal applied to the dynamic system. The system evolves its state based on this force signal and the given initial conditions, such as the robot's position and velocity at a specific time. The resulting evolution trajectory, shown as the black curve in Figure~\ref{fig:enforce_init_cond_box_push}, can be computed in closed form and used to control the robot.

When the policy is updated and predicts a new force signal for the same task, a new action trajectory is generated, depicted as the red dashed curve, which gradually deviates from the old trajectory. However, by utilizing the dynamic system's features, we can set the initial condition of each segment of the new trajectory to the corresponding old state. This ensures that the new action sequence used in the target computation in Eq.(7), can start from the old state, as shown across the five segments in the figure. Therefore, we matched the old state and new actions by eliminating the gap between them, as previously discussed in Section 4.3.1.


\begin{figure}[h]
    \centering
    \includegraphics[width=1\linewidth]{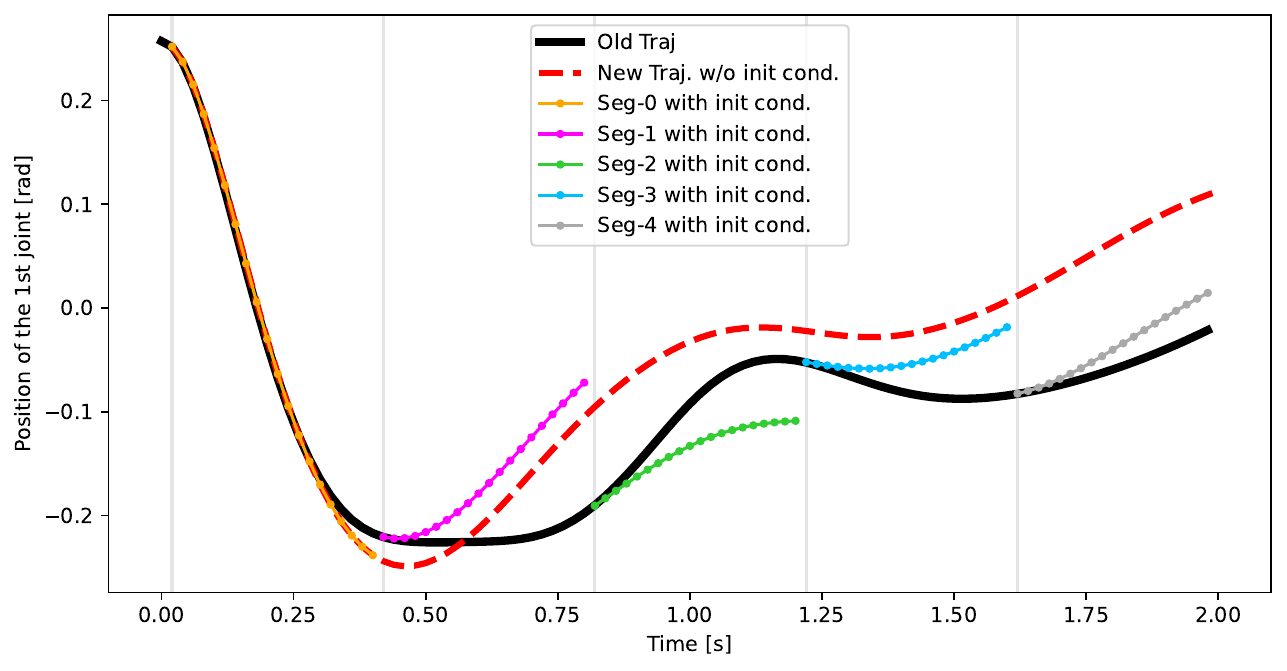}
    \caption{TOP-ERL leverages the initial condition enforcement techniques of a dynamic system to ensure that the new action trajectory starts from the corresponding old state. \textbf{These action trajectories are taken from the first DoF of the robot in the box pushing task.}}
    \label{fig:enforce_init_cond_box_push}
\end{figure}



%=================================================================
% 
%                       Policy's Training
% 
%=================================================================
\subsection{Explanation of Policy's Training additional to Section 4.4}
We utilize the transformer critic to guide the training of our policy, using the reparameterization trick similar to that introduced by SAC \citep{haarnoja2018soft}. Given a task initial state $\vs$, the current policy $\pi_{\vtheta}(\vw|\vs) \sim \mathcal{N}(\vw|\vmu_{\vw}, \mSigma_{\vw})$ predicts the Gaussian parameters of the MP's and samples $\Tilde{\vw}$ as follows:

\begin{equation}
     \hspace{-2cm}\text{Sample MP parameter vector:}~~~~~~~~~~~~~\Tilde{\vw} = \vmu_{\vw} + \mL_{\vw}\bm{\epsilon}, ~~\bm{\epsilon} \sim \mathcal{N}(\bm{0}, \bm{I}).  
     \label{eq:resample_mp}
\end{equation}

Here, $\mL_{\vw}$ is the Cholesky decomposition of the covariance matrix $\mSigma_{\vw}$, where $\mL_{\vw}\mL_{\vw}^T = \mSigma_{\vw}$. This parameterization technique is commonly used for predicting full covariance Gaussian policies. The term $\bm{\epsilon}$ is a Gaussian white noise vector with the same dimensionality as $\vw$. Eq. (\ref{eq:resample_mp}) represents the full covariance extension of the reparameterization trick typically used in RL, known as $\Tilde{a} = \mu_a + \sigma_a \epsilon,~~\epsilon \sim \mathcal{N}(0, 1)$.

The sampled $\Tilde{\vw}$ is then used to compute the new trajectory segments. Using the techniques described in Section 4.3.1 and Section R.1, we ensure each action segment $[\Tilde{\va}_t^k]_{t=0:N}$ starts from the corresponding old state $\vs_0^k$. This is achieved by enforcing the initial condition, such as the robot's position $\va$ and velocity $\dot{\va}$ at the old state.
The resulting trajectory segments are computed using the linear basis function expression in Eq. (4) from Section 3.2, where the coefficients $c_1$ and $c_2$ are determined by the initial conditions and solved using Eq. (22) in Appendix B.3:

\begin{equation}
    \hspace{-2cm}\text{Compute action segment:}~~~~~\Tilde{\va}(t) = \ipb(t)^\intercal \Tilde{\vw} + c_1y_1(t) + c_2y_2(t) \tag{4}        
\end{equation}

Here, $t=0:N$ represents the time interval from the beginning to the end of the $k$-th segment. Thus, the new action sequence $[\Tilde{\va}_t^k]_{t=0:N}$ predicted by the new policy is conditioned on both the task description and the old state. Intuitively, this can be interpreted as taking new actions for an old situation.
We evaluate and maximize the value of these action segments, using their expectation as the policy's learning objective, as shown in Eq. (9) in Section 4.4:

\begin{equation}
    \hspace{-0.3cm}\text{SAC style Objective:}~~~~~
    J(\theta) = 
    \mathbb{E}_{\vs\sim B}\mathbb{E}_{\Tilde{\vw}\sim\pi_{\theta}(\cdot|\vs)}
    \left[
    \frac{1}{KL}
    \sum_{k=1}^{K}\sum_{N=0}^{L-1}
    Q_{\phi}(\vs_0^k, \left[\Tilde{\va}_t^k\right]_{t=0:N})
    \right].
    \tag{9}
\end{equation}

Since Eq.(4), (9), (22) and (\ref{eq:resample_mp}) are all differentiable, the policy neural network parameters $\vtheta$ can be trained using gradient ascent. Compared to the technique introduced in SAC, TOP-ERL adds only one additional step: computing the action sequence $[\Tilde{\va}_t^k]_{t=0:N}$ from the sampled MP parameter $\Tilde{\vw}$.


%=================================================================
% 
%                              TRPL
% 
%=================================================================
\subsection{Technical Details of TRPL}
In Episodic Reinforcement Learning (ERL), the parameter space $\mathcal{W}$ generally has a higher dimensionality than the action space $\mathcal{A}$, creating distinct challenges for achieving stable policy updates. Trust region methods \citep{schulman2015trust, schulman2017proximal} are widely regarded as reliable techniques for ensuring convergence and stability in policy gradient algorithms.

Although methods like PPO approximate trust regions using surrogate objectives, they lack the ability to enforce trust regions precisely. To address this limitation, \citet{otto2021differentiable} proposed \TRPL, a mathematically rigorous and scalable approach for exact trust region enforcement in deep \rl algorithms. Leveraging differentiable convex optimization layers \citep{agrawal2019differentiable}, \TRPL enforces trust regions at the per-state level and has demonstrated robustness and stability in high-dimensional parameter spaces, as evidenced in methods like BBRL \citep{otto2023deep} and TCE \citep{li2024open}.

TRPL operates on the standard outputs of a Gaussian policy—the mean vector $\bm{\mu}$ and covariance matrix $\bm{\Sigma}$—and enforces trust regions through a state-specific projection operation. The adjusted Gaussian policy, represented by $\tilde{\bm{\mu}}$ and $\tilde{\bm{\Sigma}}$, serves as the foundation for subsequent computations. The dissimilarity measures for the mean and covariance, denoted as $d_\textrm{mean}$ and $d_\textrm{cov}$ (e.g., KL-divergence), are bounded by thresholds $\epsilon_\mu$ and $\epsilon_\Sigma$, respectively. The optimization problem for each state $\vs$ is expressed as:
\begin{equation}       
    \begin{aligned}
    \argmin_{\tilde{\bm{\mu}}_s} d_\textrm{mean} \left(\tilde{\bm{\mu}}_s, \bm{\mu}(\vs) \right),  \quad &\st \quad d_\textrm{mean} \left(\tilde{\bm{\mu}}_s,  \old{\bm{\mu}}(\vs) \right) \leq \epsilon_{\mu}, \textrm{ and}\\
    \argmin_{\tilde{\bm{\Sigma}}_s} d_\textrm{cov} \left(\tilde{\bm{\Sigma}}_s, \bm{\Sigma}(\vs) \right), \quad &\st \quad d_\textrm{cov} \left(\tilde{\bm{\Sigma}}_s, \old{\bm{\Sigma}}(\vs) \right) \leq \epsilon_\Sigma.   
    \end{aligned}
    \label{eq:trust_region}
\end{equation}
If the unconstrained, newly predicted per-state Gaussian parameters $\vmu(\vs)$ and $\mSigma(\vs)$ exceed the trust region bounds defined by $\epsilon_{\mu}$ and $\epsilon_{\Sigma}$, respectively, TRPL projects them back to the trust region boundary, ensuring stable update steps. In TOP-ERL, the old Gaussian parameters, $\old{\vmu}(\vs)$ and $\old{\mSigma}(\vs)$, can be derived either from the behavior policy that interacted with the environment or from an exponentially moving averaged (EMA) policy, which serves as a delayed version of the current policy. This approach is analogous to the concept employed in the target critic network.

%=================================================================
% 
%              Longer Training for Box Pushing Tasks
% 
%=================================================================
\subsection{Longer Training for Box Pushing Tasks}
In the original manuscript, we concluded the training of TOP-ERL at 14M data points in the box-pushing tasks because it clearly outperformed the baseline methods. We have now extended the training to 40M data points, as illustrated in Figure~\ref{fig:bp_40m}.
\input{figure_and_table/box_pushing_40M/__all40M__}



%=================================================================
% 
%                  Removing the Target Network
% 
%=================================================================
\subsection{Ablation: Removing the Target Network}
We conducted an ablation study by removing the target critic network in the box-pushing task under the dense reward setting and report the result in Fig. \ref{fig:ablation_no_target}. We observed poorer performance in the ablated model, highlighting the importance of the target network in our current approach. However, a recent method, Cross-Q \citep{bhatt2024crossq}, proposed several techniques leveraging batch normalization in critic updates, effectively removing the need for a target network in SAC \citep{haarnoja2018soft}. Incorporating these techniques into our transformer critic is left as future work.
\input{figure_and_table/ablation_no_target/__all_no_target__}
%=================================================================
% 
%              Effectiveness of the Critic Transformer
% 
%=================================================================
\newpage
\subsection{Ablation: Effectiveness of the Critic Transformer}
We conducted two additional ablation studies to prove the effectiveness of our transformer critic in the box pushing dense reward setting. 

\paragraph{SAC + MP}
The approach involves directly using SAC \citep{haarnoja2018soft} to predict the MP’s parameters while retaining the trajectory generation and environment rollout procedure described in Section 4.1. We sum up the rewards collected during trajectory execution and use this as the return for the entire trajectory. Here, the trajectory is treated as a single action, and the learning objective does not incorporate any temporal information within the trajectory.

\paragraph{Degenerate Critic Transformer} We degenerate our critic transformer from taking sequence of actions to a single action.
The approach retains the main architecture of TOP-ERL but reduces the segment length to one in critic updates. In this case, the transformer critic degenerates to a standard critic network, as the input consists of only one state and one action rather than a sequence of actions. 

The empirical results in Figure \ref{fig:ablation_transformer} illustrate the poor performance of both ablate approaches in the box pushing task with dense reward. For the \textbf{SAC + MP} approach, we infer that the main issue lies in its inability to leverage the temporal structure of the trajectory sequence to efficiently update the policy, making it difficult to assign credit to critical actions. This method fails to distinguish the distinct contributions of each action to task success, instead tending to average them. Additionally, the high dimensionality of the MP parameters compared to low-level actions poses challenges for Q-function learning.

For the \textbf{Degenerate Critic Transformer} method, we infer that although the action trajectory is temporally correlated, the critic fails to capture the sequence's value when only single actions are provided as input. In contrast, the default TOP-ERL model, which takes action sequences as input, effectively captures their values, leading to more efficient learning outcomes. Furthermore, we infer that using varying lengths of action sequences can implicitly regularize the training of the value function.

\input{figure_and_table/abltion_transformer/__all_critic_transformer__}

\paragraph{Impact of the Transformer-based Critic on Value Prediction.}  
To assess the impact of incorporating a transformer-based critic on value prediction, we adopt the analysis framework from Clipped Double Q-learning \citep{fujimoto2018addressing}. Specifically, we compare the average values predicted by the critics with the true values, computed using Monte Carlo returns. These findings are presented in Fig. \ref{fig:ablation_critic_value}. Additionally, we analyze the critic bias, defined as the difference between the values predicted by the critics and the Monte Carlo returns. The results, shown in Fig. \ref{fig:ablation_value_bias}, indicate that TOP-ERL consistently achieves less-biased value predictions compared to its ablated version. In contrast, a standard critic network, which only takes a single action as input, suffers from overestimation bias and often relies on additional techniques, such as Clipped Double Q-learning \citep{fujimoto2018addressing} and critic ensembles \citep{chenrandomized}, to mitigate these issues.

The advantages of using a transformer-based critic arise from several key factors. First, it processes action sequences as input, which implicitly regularizes the training of the value function. For instance, in Eq. (7), the expectation of the Q-value over $L$ actions is used as the target for the V-function prediction. By varying $L$ across different update iterations, the V-function is trained on Q-values derived from diverse action sequences, providing an implicit regularization effect on the critic network.  

Furthermore, as off-policy RL methods depend on the critic to guide policy updates, the transformer-based critic enables decision-making over action sequences rather than individual per-step actions. This capability significantly enhances training efficiency and improves task performance.

\input{figure_and_table/abltion_transformer/__all_value_error__}
\input{figure_and_table/abltion_transformer/__all_target_bias__}

% \newpage
%=================================================================
% 
%           Individual Performance of Metaworld 50 Tasks
% 
%=================================================================
\subsection{Individual Performance of Metaworld 50 Tasks}
We reported each individual Metaworld\citep{yu2020meta} task in Fig. \ref{fig:meta50_first} and Fig. \ref{fig:meta50_second}. These tasks cover a wide range of types and complexities. 
\input{figure_and_table/meta50/__all_meta50__}
